# Supplementary material for: Hybrid Spatial-Temporal Entropy Modelling for Neural Video Compression
Source: arXiv:2207.05894 source file (2022-07-13)

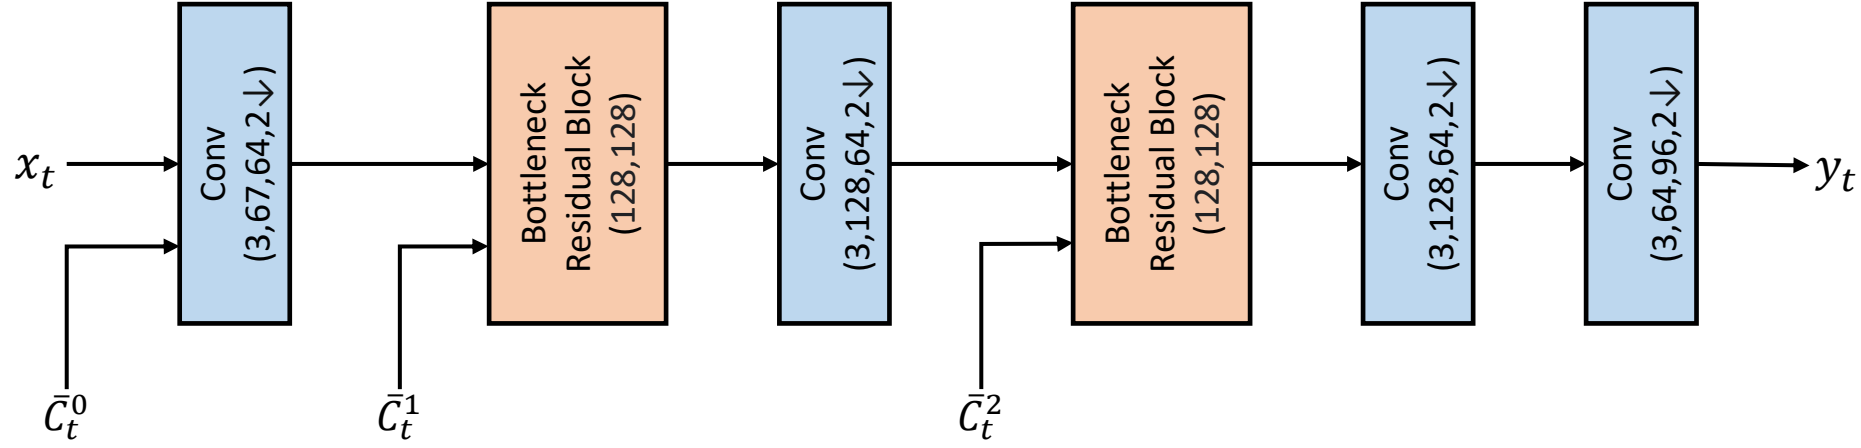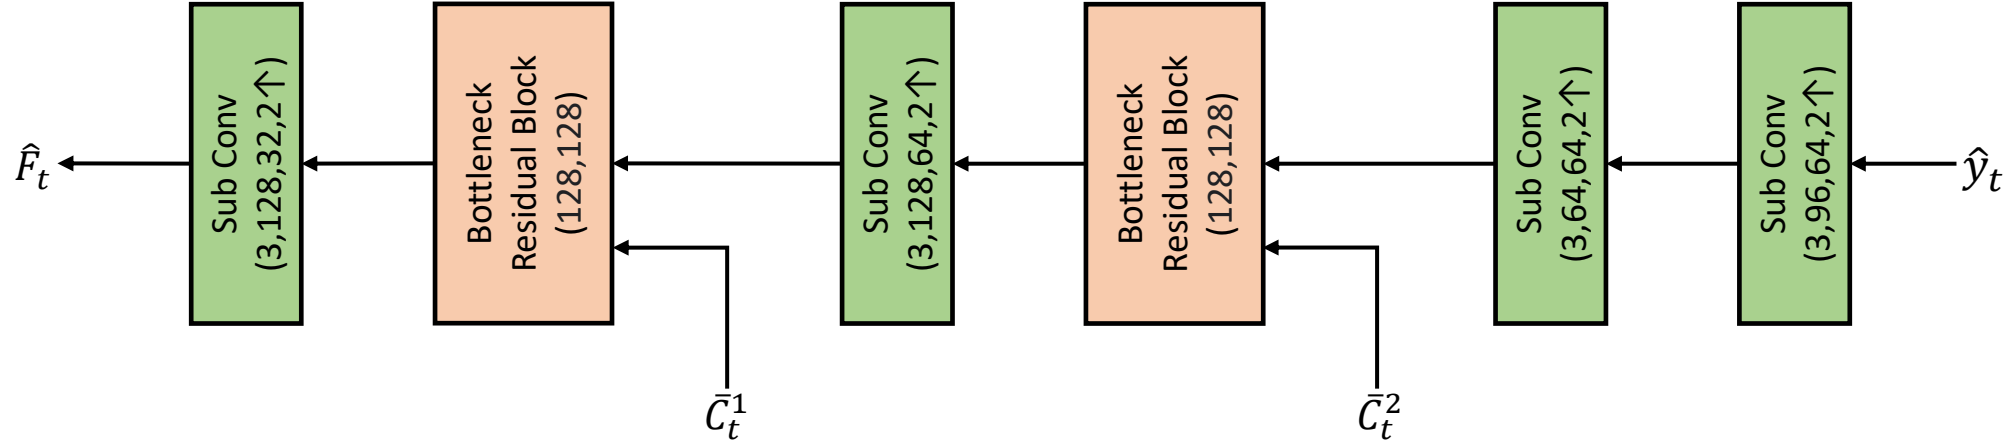

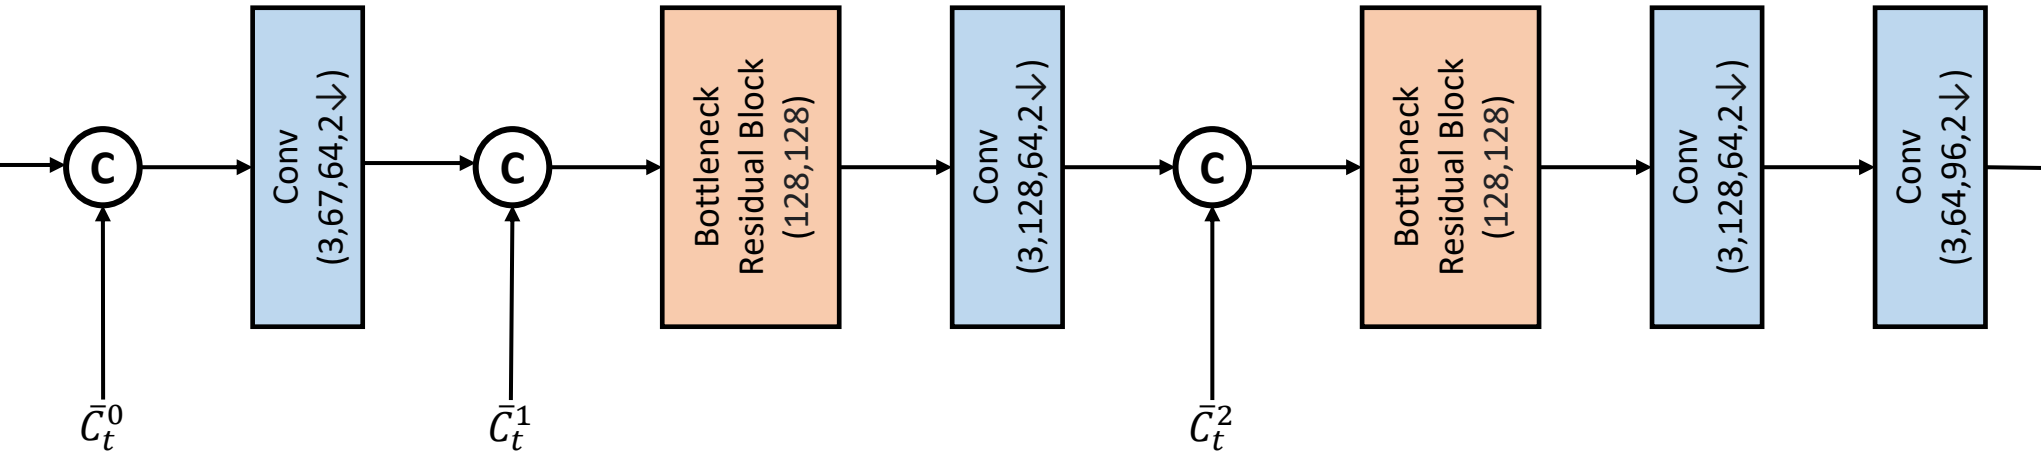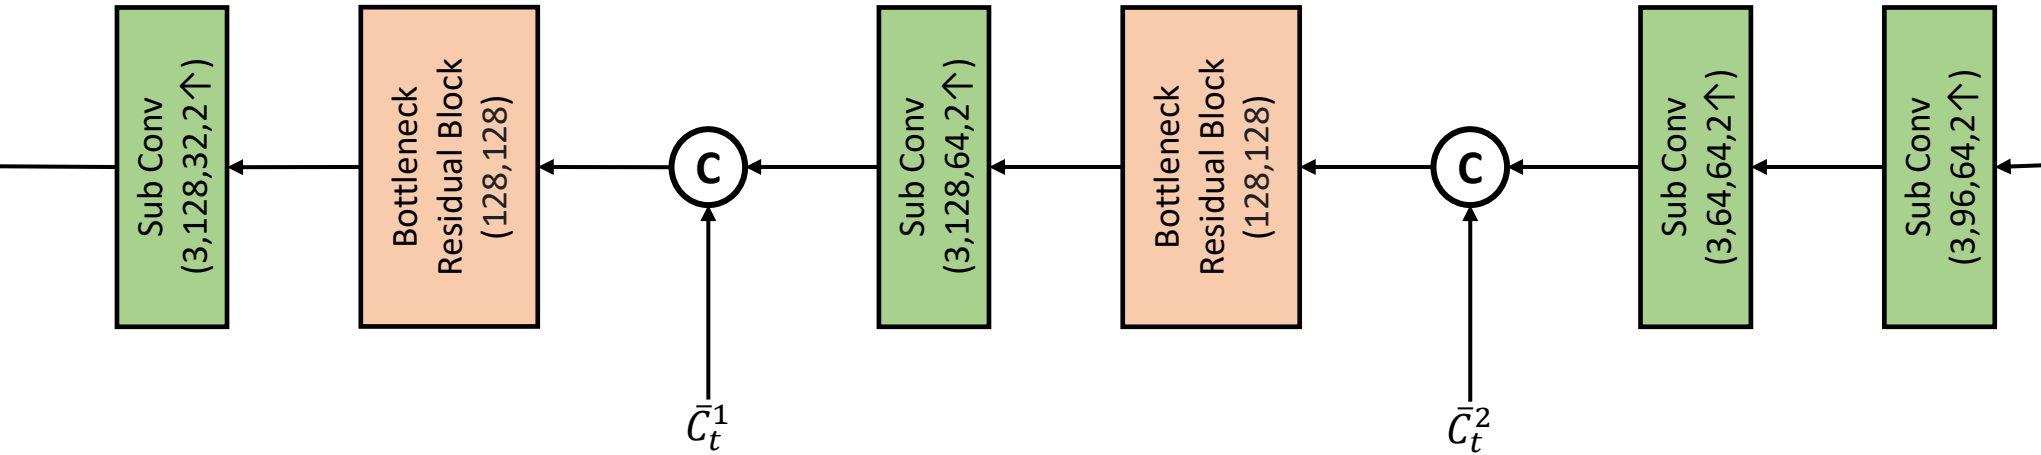

Supplement: Supplementary file 1 [file supp_contextual_encdec.pdf]
